# Supplementary material for: First-passage statistics of confined colloids
Source: arXiv:2511.11117 source file (2026-04-21)
Supplement: Supplementary file 1 [file Tournemire2025_SI.pdf]

# Non-Gaussianity-induced enhanced target-finding dynamics of confined colloids

## – Supplementary Information –

Guirec de Tournemire,<sup>1</sup> Nicolas Fares,<sup>1</sup> Yacine Amarouchene,<sup>1,\*</sup> and Thomas Salez<sup>1,†</sup>

<sup>1</sup>*Univ. Bordeaux, CNRS, LOMA, UMR 5798, F-33405 Talence, France.*

(Dated: November 14, 2025)

### LOCAL DIFFUSIVITIES

#### $z$ -dependency

Target finding is narrowly linked to the diffusivity of the system, which is characterized by a diffusion coefficient  $D_q$  (with  $q = x, z$ ). The latter is expressed through:

$$\langle \Delta_\tau q^2 \rangle = 2D_q \tau, \quad \text{with} \quad D_q = \frac{k_B \Theta}{\gamma_q}, \quad (\text{S1})$$

with  $\tau$  the lag time,  $k_B$  the Boltzmann constant,  $\Theta$  the room temperature and  $\gamma_q$  the drag term. In the absence of a wall, the bulk drag coefficient  $\gamma$  reads  $\gamma = 6\pi\eta_m a_p$ , leading to the bulk diffusion coefficient  $D_0 = k_B \Theta / \gamma$  (Stokes-Einstein relation). The relation in Eq. S1 is used to compare the experimental and theoretical Mean Square Displacements (MSD) shown in Fig. 1d of the main document. The latter observable provides an estimation of the reduced diffusion coefficient  $D_q$ , deduced when  $\tau < \tau_{\text{eq}}$  (the equilibrium time defined in the main document). More precisely, the no-slip boundary condition at the substrate ( $z = 0$ ) reduces the colloid's diffusivity. Besides, the anisotropy of the colloid's motion recasts into a smaller average diffusion coefficient in the vertical direction as compared to the horizontal one ( $D_z < D_x$ ). Furthermore, the aforementioned diffusion and drag coefficients are actually averaged over all colloid-wall gap distances  $z$ . However, the hydrodynamic drag felt by the colloid is in fact  $z$ -dependent. This hydrodynamic drag increases as the colloid approaches the surface, as accurately described within the theoretical frameworks developed by Faxén [1] and Brenner [2], which respectively account for the in-plane and perpendicular drags acting on the colloid. This leads to altitude-dependent local diffusion coefficients  $d_q$ . The altitude dependency of the parallel diffusion coefficient  $d_x$  reads:

$$d_x = D_0 \left( 1 - \frac{9}{16}Z + \frac{1}{8}Z^3 + \frac{45}{256}Z^4 + \frac{1}{16}Z^5 \right), \quad \text{with} \quad Z = \left( \frac{a_p}{a_p + z} \right). \quad (\text{S2})$$

The one of the perpendicular diffusion coefficient  $d_z$ , within the Padé approximation (leading to a 1% accuracy), reads:

$$d_z = D_0 \left( \frac{6z^2 + 2a_p z}{6z^2 + 9a_p z + 2a_p^2} \right). \quad (\text{S3})$$

The theoretical and experimental  $z$ -dependencies of these local diffusion coefficients  $d_q$  are shown in Fig. S1.

#### Inference of local diffusion coefficients

The determination of the local diffusion coefficients  $d_q$  with nanometric spatial precision requires going beyond simple spatial binning. Indeed, conventional binning approaches, which are suitable for static observables, fail to capture the subtle variations of dynamic quantities such as local diffusion. To overcome this limitation, the experimental profiles of the local diffusion coefficients presented in Fig. S1 are obtained using a Stochastic Force Inference (SFI) algorithm [3]. This method combines statistical inference with trajectory analysis to extract diffusion properties even in the presence of measurement noise.

An unbiased estimator  $\hat{\delta}$  of the local diffusion coefficient in the  $x$ -direction (which can be straightforwardly extended to the  $z$ -direction) is defined as:

$$\hat{\delta} = \frac{(\Delta_\tau x(t_{j-1}) + \Delta_\tau x(t_j))^2}{4\tau} + \frac{\Delta_\tau x(t_{j-1}) \Delta_\tau x(t_j)}{2\tau}, \quad (\text{S4})$$

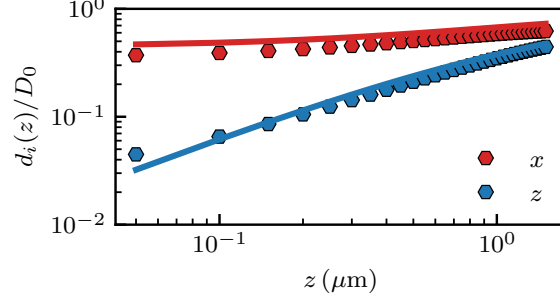

FIG. S1: Local diffusion coefficients in both the perpendicular (blue hexagons) and in-plane (red hexagons) directions, as a function of the wall-colloid gap distance  $z$ , for a spherical polystyrene colloid of radius  $a_p = 1.48 \mu\text{m}$  diffusing in water, of viscosity  $\eta_m = 0.95 \text{ mPa}\cdot\text{s}$ , near a rigid glass wall. Theoretical predictions from Eq. S3 (blue line) for the perpendicular diffusion coefficient and Eq. S2 (red line) for the parallel diffusion coefficient are also shown.

where  $\tau$  represents an integer multiple of the sampling acquisition rate ( $dt = 1/\text{fps}$ ), and  $\Delta_\tau x(t_j)$  denotes the colloid displacement over a time interval  $\tau$  starting at time  $t_j$ . Each estimator value  $\hat{d}$  corresponds to a specific height  $z$ , and its spatial distribution is reconstructed on a regular grid  $\hat{z}$  through polynomial interpolation of the form  $\sum a_k(\hat{z})z^k$ , where  $a_k$  are real coefficients. In this work, polynomial bases of third or fourth order are employed, while truncating at  $k = 0$  corresponds to the conventional binning approach.

The two terms in Eq. S4 serve distinct purposes. The first corresponds to the classical definition of the diffusion coefficient in the 2D case (see Eq. S1), while the second acts as a corrective term compensating for noise-induced correlations in experimental data. In an ideal Brownian process, successive displacements  $\Delta_\tau x$  are delta-correlated. However, measurement errors violate this assumption, introducing spurious correlations. Incorporating the autocorrelation term (second term in Eq. S4) therefore isolates the true diffusive behavior from noise artifacts, yielding an unbiased estimator. Under the present experimental conditions, this correction is essential for obtaining accurate local diffusion coefficients near the substrate ( $z \leq 100 \text{ nm}$ ), where data are limited due to electrostatic repulsion, and where statistical fluctuations are most pronounced due to the increased dissipation therein.

### TUNING THE CONFINEMENT

In order to choose a given confinement strength for the colloid, we use the following procedure. The upper boundary of the confinement is set by the Boltzmann length  $l_B$ , as shown in Fig. 1f of the main document. Indeed, the typical altitude at which the colloid starts to feel the confinement due to gravity is expressed as:

$$l_B = \frac{k_B \Theta}{\Delta m g}, \quad \text{with} \quad \Delta m = \frac{4}{3} \pi a_p^3 \Delta \rho = \frac{4}{3} \pi a_p^3 (\rho_p - \rho_m), \quad (\text{S5})$$

with  $a_p$  the radius of the colloid, and  $\rho_p$  and  $\rho_m$  respectively the density of the colloid and the density of the medium. Consequently, tuning the density of the mixture  $\rho_m$ , through the addition of one fluid element, would lead to a different Boltzmann length  $l_B$ , *i.e.* a different confinement. Two side effects of this experimental method are to be noticed:

- (i) it affects the optical index of the medium  $n_m$ , which is involved in our monitoring method.
- (ii) it changes as well the viscosity of the medium  $\eta_m$ , inducing a modification of the bulk diffusion coefficient.

A detailed explanation on how one can overpass these two subtleties is detailed hereafter.

(i) Since the holography method we use partly relies on the optical-index difference between the monitored object and its environment, a modification in these optical indices would lead to a misinterpretation of the observables. In order to avoid any confusion between the different experiments, optical indices are pre-calibrated using a refractometer (DR-M2/1550 from ATAGO). A table listing optical indices, as a function of the Ethylene Glycol weight ration  $W_{EG}$ , is shown in Table S1.

| $W_{\text{EG}} \%$                         | 42     | 30     | 0      |
|--------------------------------------------|--------|--------|--------|
| $n(\lambda = 500\text{nm})$                | 1,3769 | 1,3690 | 1,3350 |
| $n(\lambda = 600\text{nm})$                | 1,3735 | 1,3663 | 1,3323 |
| $n(\lambda_{\text{laser}} = 532\text{nm})$ | 1.3705 | 1.3681 | 1.3341 |

TABLE S1: Optical indices of the solution which contains the diffusing colloid, as functions of the ethylene-glycol-water solution's weight ratio  $W_{\text{EG}}$  in ethylene glycol.

(ii) The Boltzmann length  $l_{\text{B}}$  as a function of the density difference  $\Delta\rho$  is straightforwardly expressed in Eq. S5. Subsequently, we aim to cover a couple of decades in  $l_{\text{B}}$  to have a thorough understanding of the influence of confinement on the FPTD, ranging from few tens of nm to the bulk case ( $l_{\text{B}} \rightarrow \infty$ ).

| $W_{\text{EG}} (\%)$ | $\eta_m$ (mPa.s) | $\rho_m$ (kg/m <sup>3</sup> ) | $\rho_p$ (kg/m <sup>3</sup> ) | $\Delta\rho$ (kg/m <sup>3</sup> ) | $a$ ( $\mu\text{m}$ ) | $l_{\text{B}}^{\text{th}}$ (nm) | $l_{\text{B}}^{\text{exp}}$ (nm) |
|----------------------|------------------|-------------------------------|-------------------------------|-----------------------------------|-----------------------|---------------------------------|----------------------------------|
| 42                   | 3.2              | 1050                          | 1050                          | 0                                 | 1.48                  | $+\infty$                       | $+\infty$                        |
| 30                   | 2.10             | 1033                          | 1050                          | 17                                | 1.47                  | 1787                            | 1802                             |
| 0                    | 0.95             | 1000                          | 1050                          | 50                                | 1.48                  | 596                             | 604                              |
| 30                   | 2.10             | 1033                          | 1050                          | 17                                | 2.98                  | 215                             | 204                              |
| 0                    | 0.95             | 1000                          | 1050                          | 50                                | 2.98                  | 73                              | 79                               |

TABLE S2: List of the Boltzmann lengths  $l_{\text{B}} = [79 \text{ nm}, 204 \text{ nm}, 604 \text{ nm}, 1802 \text{ nm}, +\infty]$  obtained from different ethylene-glycol-water mixtures of ethylene-glycol weight ratios  $W_{\text{EG}}$ , for two radii  $a_{\text{p}}$  of the colloid.

First, the good agreement, detailed in Tab. S2, between the theoretical (Eq. S5) and experimental (deduced from the best fit of the experimental  $P_{\text{eq}}(z)$  to Eq. 1 of the main document) Boltzmann lengths serves as a validation of our method. Second, one can notice that as the ethylene-glycol weight ratio  $W_{\text{EG}}$  in the mixture increases, the mixture's dynamic viscosity  $\eta_m$  increases as well. This would lead to different bulk diffusion coefficients  $D_0$  (see Eq. S1), hence a different effective diffusion coefficient  $D_x$  (see Eq. S2), for each experiment, preventing any possible comparison between bulk and confined FPTDs. This hurdle, and the will to generalize the results to any distance  $L$  to the target, suggest the use of rescaled and dimensionless variables accounting for the change of diffusion coefficient, as:

$$T = \frac{D_0 t}{L^2} \quad ; \quad F(T) = f(T) \frac{L^2}{D_0}. \quad (\text{S6})$$

Remark: For bulk and quasi-bulk experiments ( $l_{\text{B}} \rightarrow +\infty$  and  $l_{\text{B}} = 1802 \text{ nm}$  respectively), some of the observables struggled to converge, as for instance  $P_{\text{eq}}(z)$ , since the equilibrium time  $\tau_{\text{eq}}$  gets greater as  $l_{\text{B}}$  increases. In these cases, the MSD was the most suitable observable to deduce information on confinement.

## STATISTICAL OPTIMIZATION ALGORITHM

In order to optimize the statistical reliability of our experimental and numerical data, an optimization has been performed in agreement with the theory. Indeed, we use an experiment which contains an entire trajectory as a group of many trajectories, as follows: one first-passage time (FPT) is extracted when a colloid starting at  $q = q(t=0) = q_0$  (where  $q = x, z$ ) reaches  $q = q_0 + L$ . The workaround resides in considering successively every position as an initial position  $q_0$ : the first initial position  $q_0 = q(t=0)$  leads to the first FPT, the second initial position  $q_0 = q(t=\tau)$  leads to the second FPT, and so on ... until the FPT of the  $n^{\text{th}}$  initial position  $q_0 = q[t = (n-1)\tau]$  is never reached because of the end of the recording. By applying this algorithm, one can infer from a single trajectory a well-converged distribution as shown in Figs. 2b, 3a and 4a of the main document. We stress that, in the case of a wall-normal target search along  $z$ , the initial positions  $z_0$  are selected from the equilibrium distribution  $P_{\text{eq}}(z)$  (see Fig. 1c of the main document).

## LANGEVIN SIMULATIONS

Numerical simulations are conducted based on the Langevin equations presented in the main text (see Eqs. (7,12)), which are discretized using a numerical integration time step of 10 ms. This time step is selected to match the experimental acquisition frame rate. All associated simulation codes are openly accessible at [https://github.com/EMetBrown-Lab/Numerical\\_simulations\\_of\\_confined\\_brownian\\_motion/tree/main/Double\\_Walls\\_Overdamped\\_Langevin\\_Python/](https://github.com/EMetBrown-Lab/Numerical_simulations_of_confined_brownian_motion/tree/main/Double_Walls_Overdamped_Langevin_Python/). After downloading the necessary scripts (see `simulations/langevin`) and installing standard Python libraries, confined Brownian trajectories can be generated using the following code snippet:

```

1  from simulations.langevin.DoubleWalls_Overdamped_Langevin import DoubleWallsLangevin
2  def compute_one_traj(i, dt, Nt, Nt_sub, a, H, lD, lB, B, etam, T, R0=None):
3      brown = DoubleWallsLangevin(
4          dt=dt_num, Nt=Nt, Nt_sub=Nt_sub,
5          a=a, H=H, lD=lD, lB=lB, B=B, etam=etam, T=T,
6          R0=R0,
7      )
8      brown.trajectory()
9      x = brown.Xn
10     z = brown.Zn + H
11     return x, z
12 x, z = compute_one_traj(i, dt, Nt, Nt_sub, a, H, lD, lB, B, etam, T, R0=None)

```

FIG. S2: Code snippet to generate confined Brownian trajectories.

In order of appearance, the input variables of the function `compute_one_traj` are defined as follows: an integer index (used when the function is executed within a loop), the numerical integration time step, the total number of simulated points  $N_{\text{tot}}$ , the sub-sampling factor, the colloid radius  $a_p$ , half-length  $H$  of the inter-wall separation  $2H$  within the confining chamber, the Debye length  $l_D$ , the Boltzmann length  $l_B$ , the dimensionless amplitude  $B$  of the electrostatic repulsion (expressed in units of  $k_B\Theta$ ), the dynamic viscosity of the medium  $\eta_m$ , the temperature  $\Theta$ , and the initial position ( $x_0 = x(t=0)$ ,  $z_0 = z(t=0)$ ) of the colloid. Further details concerning the simulation procedure are provided in Ref. [4].

## RELATIVE TIME DELAY

In order to quantify the time shift between the bulk and confined FPTDs, as the colloid searches for a target in the direction parallel to the wall, we build a dimensionless rescaled time shift, detailed hereafter. In the case of a colloid searching a target placed along  $x$  (or along  $y$ ), its most likely first-passage time can be deduced from the time derivative of its FPTD, as:

$$\frac{dF(T)}{dT} = 0 \quad \text{for} \quad T = T^{\text{max}}. \quad (\text{S7})$$

This general consideration leads to:

$$T^{\text{max}} = \frac{L^2}{6D}, \quad (\text{S8})$$

with  $D$  the coefficient of the colloid in its environment. In the case of confined diffusion, this diffusion coefficient exhibits a  $z$ -dependency, as mentioned at the beginning of this Supplementary Information

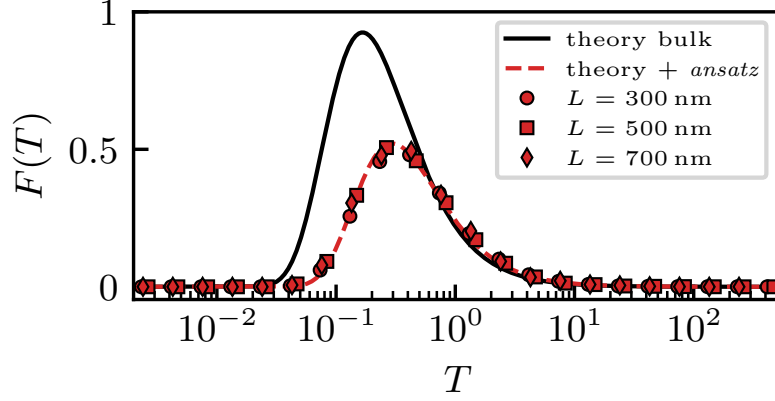

FIG. S3: First-passage-time distribution for a confined polystyrene colloid with a radius  $a_p = 1.5 \mu\text{m}$  in water ( $D_0 = 15.1 \cdot 10^{-2} \mu\text{m}^2/\text{s}$ ), for a target placed at a distance  $L = [300 \text{ nm}, 500 \text{ nm}, 700 \text{ nm}]$  (along  $x$ ) from the initial position  $x = x_0$ .

document. The quantity we aim to characterize is the dimensionless rescaled time shift  $\frac{\Delta T^{\max}}{T_{\text{bulk}}^{\max}}$  and is expressed as:

$$\frac{\Delta T^{\max}}{T_{\text{bulk}}^{\max}}(z, a_p) = \frac{D_0}{d_x(z, a_p)} - 1. \quad (\text{S9})$$

Since we showed that a Levy distribution containing an *ansatz* that sets the local diffusion coefficient  $d_x$  to its average value  $D_x$  (see Eqs. 5 and 13 of the main document) is a valid approximation (see Fig. 3a of main document), one has:

$$\frac{\Delta T^{\max}}{T_{\text{bulk}}^{\max}}\left(\frac{a_p}{l_B}\right) = \int_0^{+\infty} dz P_{\text{eq}}(z, B, l_D, l_B) \left[ \frac{D_0}{d_x(z, a_p)} - 1 \right]. \quad (\text{S10})$$

From this integral, one can deduce using *e.g.* Mathematica,  $\frac{\Delta T^{\max}}{T_{\text{bulk}}^{\max}}$  as function of the confinement parameter  $\Lambda = \frac{a_p}{l_B}$ .

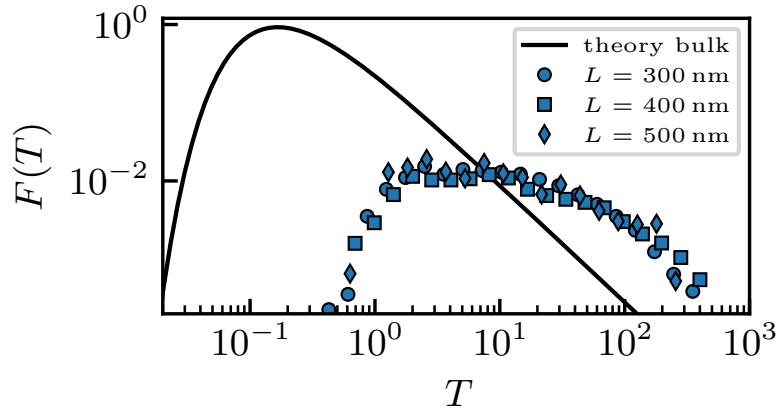

FIG. S4: First-passage-time distribution for a confined polystyrene colloid with a radius  $a_p = 3 \mu\text{m}$  in water ( $D_0 = 7.53 \cdot 10^{-2} \mu\text{m}^2/\text{s}$ ), for a target placed at a distance  $L = [300 \text{ nm}, 400 \text{ nm}, 500 \text{ nm}]$  (along  $z$ ) from the initial position  $z_0$ , where the latter is randomly selected from the equilibrium distribution  $P_{\text{eq}}$ .

## INFLUENCE OF THE DISTANCE TO THE TARGET

Here, we discuss the influence of the distance  $L$  between the initial position  $q_0$  and the target placed at  $q_0 + L$ . One can notice the fair agreement between the rescaled FPTDs, obtained for different distances  $L = [300 \text{ nm}, 500 \text{ nm}, 700 \text{ nm}]$  and  $[300 \text{ nm}, 400 \text{ nm}, 500 \text{ nm}]$ , for search processes respectively along  $x$  as shown in Fig. S3, and along  $z$  as shown in Fig. S4. Hence, the proposed variable rescaling captures de  $L$ -dependency.

---

\* yacine.amarouchene@u-bordeaux.fr

† thomas.salez@cnrs.fr

- [1] H. Faxen, Die bewegung einer starren kugel längs der achse eines mit zäher flüssigkeit gefüllten rohres, Arkiv for Matematik Astronomi och Fysik **17**, 1 (1923).
- [2] H. Brenner, The slow motion of a sphere through a viscous fluid towards a plane surface, Chemical engineering science **16**, 242 (1961).
- [3] A. Frishman and P. Ronceray, Learning force fields from stochastic trajectories, Physical Review X **10**, 021009 (2020).
- [4] E. Millan, M. Lavaud, Y. Amarouchene, and T. Salez, Numerical simulations of confined brownian-yet-non-gaussian motion, The European Physical Journal E **46**, 24 (2023).
